# Supplementary material for: Room temperature two-dimensional antiferromagnetic Weyl semimetal CrO with giant spin-splitting and spin-momentum locked transport
Source: arXiv:2104.07390 ancillary file (2021-04-19)
Supplement: Supplementary file 1 [file SI.pdf]

*Support Information for*

# Two-dimensional CrO: a collinear antiferromagnetic Weyl semimetal with spin-polarized transportation

Xin Chen[1], Duo Wang[1], Linyang Li [2,*], and Biplab Sanyal [1,*]

[1]Department of Physics and Astronomy, Uppsala University, Box 516, 751 20 Uppsala, Sweden

[2]School of Science, Hebei University of Technology, Tianjin 300401, China

Corresponding authors:

*Email: linyang.li@hebut.edu.cn (L. L.)

*Email: biplab.sanyal@physics.uu.se (B. S.)

## I. The determination of the U value

We determined the U value in this workflow:

Step 1. Fully optimize the structure using LSDA without U correction.

Step 2. Do self-consistent calculation using HSE06 functional, and get the atomic magnetic moment of Cr atoms $\mathrm{M_H}$.

Step 3. Do self-consistent calculations using the LSDA+U method with different U values to get the atomic magnetic moment function of Cr atoms $\mathrm{M_U(U)}$.

Step 4. Let $\mathrm{M_U(U) = M_H}$, and get the U value.

From these calculations, we determined the U value as U=3.55 eV.

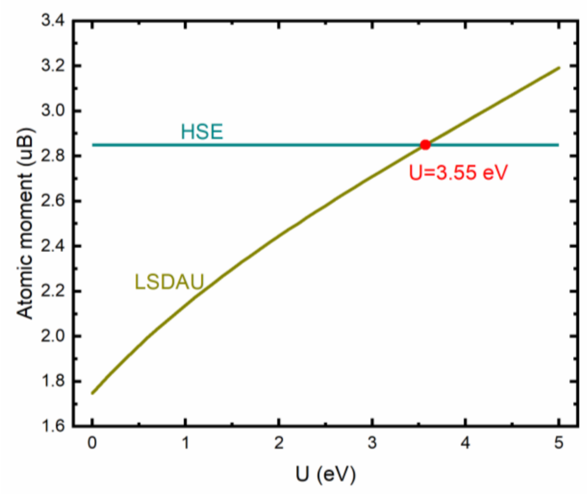


Figure S1 The atomic magnetic moments as a function of U values. The atomic magnetic moment getting from HSE06 calculation is illustrated by the dark green horizontal line.

II. The magnetic configurations

Three magnetic configurations have been considered, i.e., FM, AFM1, and AFM2, as shown in Figure S2 (a). The energy differences between the AFM2 or FM magnetic orders and the AFM1 order, $\Delta E$, are computed using different U values, as shown in Figure S2 (b). It is observed that the AFM1 is always the ground state when the U value is smaller than 5 eV.

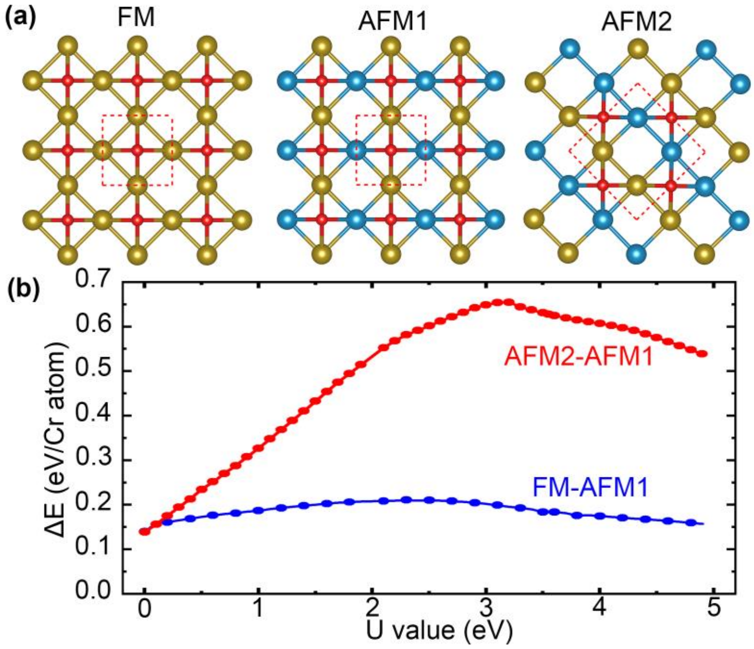


Figure S2 (a) The three magnetic configurations are considered. The red balls are oxygen atoms, the brown balls are Cr atoms with the spin-up magnetic moments, and the blue balls are the Cr atoms with spin-down magnetic moments. (b) The energy difference between the AFM1 states and the two metastable states.

III. The stability of AFM s-CrO in structure

The structural stability is confirmed by the phonon spectrum and BOMD calculations, as shown in Figure S3. There is no imaginary frequency in the phonon spectrum. In the BOMD simulation at 300 K, the energies are kept stable, and there are no obvious structural changes after heated.

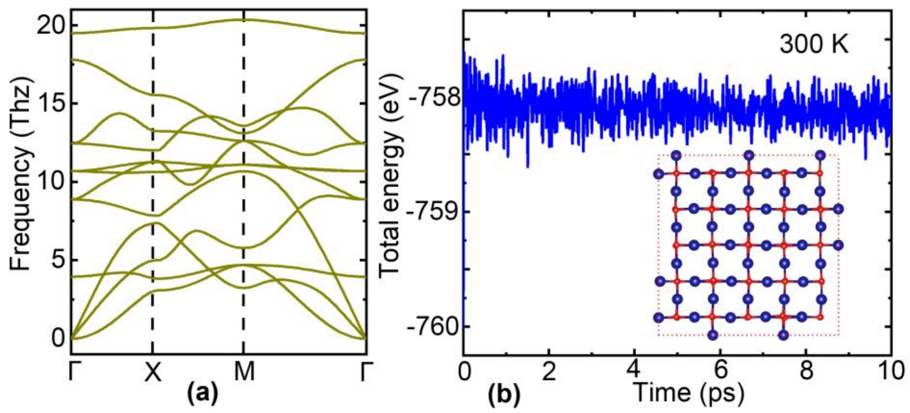


Figure S3 (a) the phonon spectrum of AFM s-CrO. (b) The energy changes in the BOMD simulation at 300 K up to 10 ps. The final heated structure is also shown.

IV. The magnon dispersion spectra without SOC

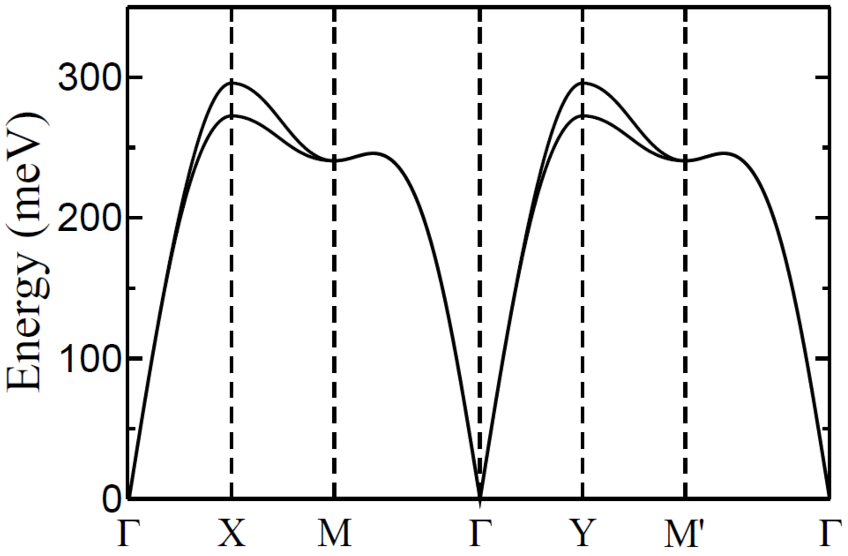


Figure S4 The magnon dispersion spectra of monolayer CrO without considering the SOC effect.

V. The 3D electronic band structures near the Fermi level

The electronic dispersion near the Fermi level is also shown in the 3D electronic band structures in Figure S4.

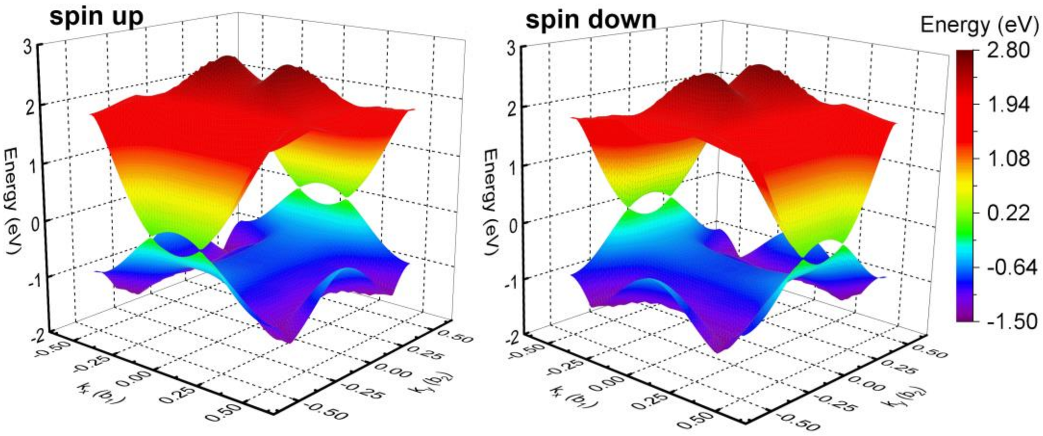


Figure S5 The electronic band structures in the first BZ in both spin channels.

VI. The PDOS of AFM s-CrO monolayer

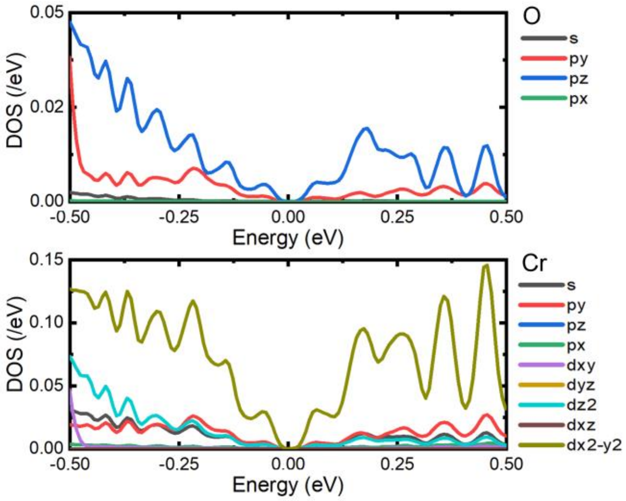


Figure S6 The PDOS of s-CrO. The up and down panels show the PDOS of each atomic orbitals of Cr and O atoms, respectively. All the atomic orbitals are illustrated in different colors.

VII. The electronic band structures with SOC effect

The band structures with the SOC effect are shown in Figure S7. As shown in Figure (b), there no bandgap opened at the Fermi level. With the in-plane magnetic axis, the degeneracy of the bands in the red rectangle in Figure S7 (c) is lifted.

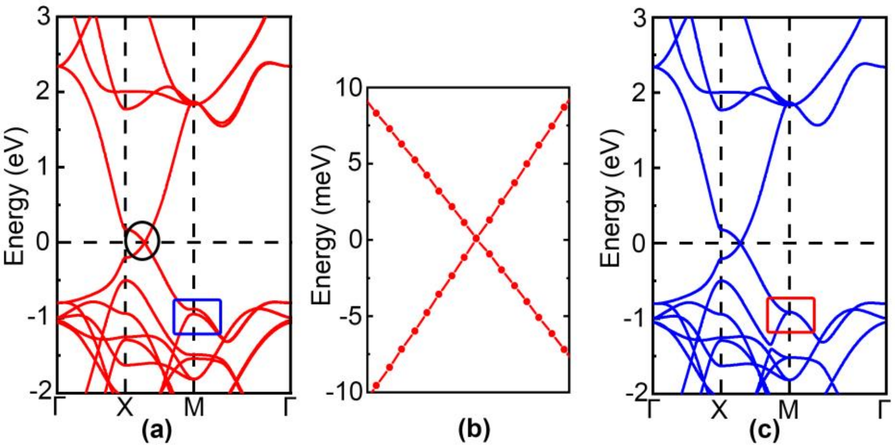


Figure S7 The band structures with SOC effect with the magnetic axis along (a) the x-direction and (c) the z-direction. The Weyl points in the black circle are enlarged and shown in (b). The band splitting in the blue rectangle is generated from the in-plane magnetic axis.

VIII. Spin density distribution in AFM s-CrO with and without strain

Due to the broken of symmetry, the sum of the atomic magnetic moments of two Cr atoms in a unit cell is not zero under an unequal-biaxial strain, as shown in Figure S8A (a). However, the total magnetic moment of a unit cell is usually zero, as shown in Figure S8A (b). This can be confirmed by looking at their band structures. The extra magnetic moments which cancel with the net magnetic moment of Cr atoms is actually from oxygen atoms. As shown in Figure S8B (a), the spin-up and spin-down charge around an oxygen atom is symmetric by a 90-degree rotation operator without unequal-biaxial strain. With strain (0%, 9%), the symmetry is broken, there are more spin-up charges around oxygen atoms, which cancel with the spin-down net magnetic moments of Cr atoms, giving rise to zero total magnetic moments.

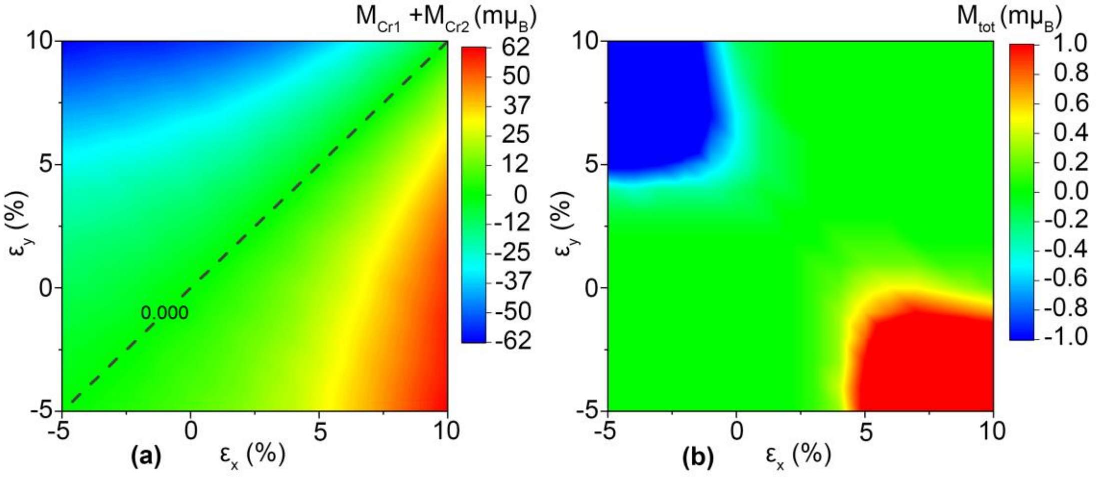


Figure S8A (a) The sum of the atomic magnetic moment of two Cr atoms with opposite spin polarization, $\mathrm{M_{Cr1}}$ and $\mathrm{M_{Cr2}}$. (b) The total magnetic moment of a unit cell of AFM s-CrO.

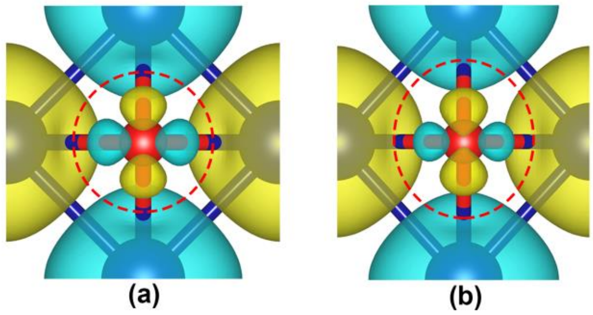


Figure S8B The spin density distribution of AFM s-CrO (a) without strain, and (b) with the unequal-biaxial strain of (0%, 9%). Spin-up and spin-down charges are in yellow and blue, respectively. The isosurface value is 0.008 e.

IX. Potential applications in spintronics

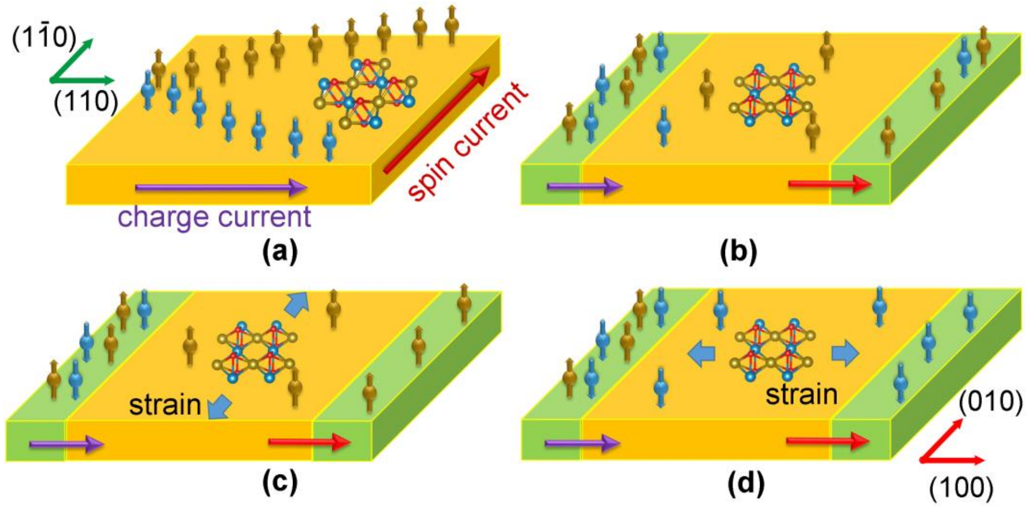


Figure S9 (a) The crystal spin Hall effect and induced spin current. Spin-polarized transportation and spin-polarized current (b) without and with tensile strain along (c) the vertical and (d) the horizontal direction. The green compass is for Figure (a), and the red compass is for Figures (a), (b), and (c).
